# Supplementary material for: Nuclear three-body short-range correlations in coordinate space
Source: arXiv:2301.09605 source file (2023-01-23)
Supplement: Supplementary file 1 [file 3N_SRC_coordinate_space_SUPP_MATERIAL_23012023.pdf]

# Nuclear three-body short-range correlations in coordinate space - Supplemental Material

Ronen Weiss[1] and Stefano Gandolfi[1]

[1] *Theoretical Division, Los Alamos National Laboratory, Los Alamos, New Mexico 87545, USA*

(Dated: January 23, 2023)

## I. THREE-BODY UNIVERSAL FUNCTIONS AND DOMINANT CHANNELS

In the paper we presented the asymptotic factorization of a many-body nuclear wave function for the case of short-range correlated (SRC) triplets. This factorization involves the universal three-body function $\varphi^{\beta}_{ijl}(\boldsymbol{x}_{ij}, \boldsymbol{x}_{ijl})$, defined as a zero-energy solution of the three-body Schrödinger equation with quantum numbers given by $\beta$. We provide here more details regarding the structure of $\varphi^{\beta}_{ijl}$ and the dominant three-body channels $\beta$.

For nuclear interactions, as mention in the paper, each channel $\beta$ is defined by the triplet quantum numbers

$$\beta = (\pi_\beta, j_\beta, m_\beta, t_\beta, t_{z,\beta}). \tag{1}$$

Generally, $\varphi^{\beta}_{ijl}$ can be written in the following way

$$\varphi^{\beta}_{ijl}(\boldsymbol{x}_{ij}, \boldsymbol{x}_{ijl}) = \hat{\mathcal{A}} \sum_{[k]\equiv \ell_1,\ell_2,\ell,s_x,s,t_x} \phi^{\beta}_{[k]}(x_{ij}, x_{ijl}) \eta^{t_x}_{t_\beta,t_{z,\beta}} [Y_{(\ell_1,\ell_2)\ell}(\hat{x}_{ij}, \hat{x}_{ijl}) \otimes \chi^{s_x}_{s}]^{j_\beta,m_\beta}. \tag{2}$$

In this expression, the angular part is given by

$$Y_{(\ell_1,\ell_2)\ell m}(\hat{x}_1, \hat{x}_2) = [Y_{\ell_1}(\hat{x}_1) \times Y_{\ell_2}(\hat{x}_2)]^{\ell m}. \tag{3}$$

It is coupled to a three-nucleon spin function $\chi^{s_x}_{sm_s}$, defined by coupling the spin of particles $i$ and $j$ to $s_x$ (0 or 1), which is then coupled to the spin of particle $l$ to create the three-nucleon spin $s$ and it projection $m_s$. $\eta^{t_x}_{t_\beta,t_{z,\beta}}$ is the three-nucleon isospin function, defined similarly. $\phi^{\beta}_{[i]}$ depends on the vector magnitudes $x_{ij} = |\boldsymbol{x}_{ij}|$ and $x_{ijl} = |\boldsymbol{x}_{ijl}|$; it does not depend on $m_\beta$ or $t_{z,\beta}$ (assuming isospin symmetry for the latter). The sum over $\ell_1, \ell_2$ is restricted to values that respect the parity, i.e. $(-1)^{\ell_1+\ell_2} = \pi_\beta$ (notice that $\phi^{\beta}_{[i]}$ is unchanged under reflection). Notice that generally the parity of $\ell$ does not determine the parity of $\varphi^{\beta}_{ijl}$. But, for the case of $\ell = 0$, for which only $\ell_1 = \ell_2$ pairs contribute, the parity is positive. $\hat{\mathcal{A}}$ is the anti-symmetrization operator.

The anti-symmetrization leads to a constrain on some of the quantum numbers in the sum over $[k]$ for this form of the wave function. The exchange of particles $i$ and $j$ leaves $x_{ij}$ unchanged, $\hat{x}_{ij}$ gets a minus sign, and $\boldsymbol{x}_{ijl}$ is unchanged. Therefore, $\phi^{\beta}_{[k]}$ is unchanged under this permutation and $Y_{(\ell_1,\ell_2)\ell}$ gets a factor of $(-1)^{\ell_1}$. $\chi^{s_x}_{s,s_z}$ and $\eta^{t_x}_{t,t_z}$ obtain a factor of $(-1)^{s_x+1}$ and $(-1)^{t_x+1}$, respectively. Thus, we conclude that if the sum $\ell_1 + t_x + s_x$ is even the corresponding component of the wave function cannot be anti-symmetrized, i.e. this component will not survive the action of $\hat{\mathcal{A}}$. Therefore, only combinations with odd $\ell_1 + t_x + s_x$ contribute in the sum over $[k]$.

For three particles close to each other we expect channels that include an $\ell = 0$ component, and specifically an $\ell_1 = \ell_2 = 0$ component, to be dominant. As mentioned above, $\ell = 0$ is possible only for the case of positive parity $\pi_\beta = +$. In addition, since the spin is either $s = 1/2$ or $s = 3/2$, it is possible to have an $\ell = 0$ component only for $j_\beta = 1/2$ or $j_\beta = 3/2$. Notice that for $j_\beta = 3/2$, the component with $\ell = 0$ must be coupled to $s = 3/2$, which means that $s_x = 1$. If we consider the $\ell_1 = \ell_2 = 0$ component, then the restriction that $\ell_1 + t_x + s_x$ is odd means that $t_x = 0$, which implies that only $t_\beta = 1/2$ is possible for $j_\beta = 3/2$. Therefore, for $t_\beta = 1/2$ triplets we have both $j^\pi = \frac{3}{2}^+$ and $j^\pi = \frac{1}{2}^+$, but for $t_\beta = 3/2$ we are left only with $j^\pi = \frac{1}{2}^+$.

We can look more carefully on the $\ell_1 = \ell_2 = 0$ component for the above options. For $t_\beta = 3/2$ and $j^\pi = \frac{1}{2}^+$, the wave function is of the form $\hat{\mathcal{A}}\phi^{\beta}_{[k]}(x_{ij}, x_{ijl})\eta^{t_x=1}_{\frac{3}{2},t_{z,\beta}}\chi^{s_x=0}_{s=1/2,m_\beta}$ (using the constrain on $\ell_1 + t_x + s_x$). $\eta^{t_x=1}_{\frac{3}{2},t_{z,\beta}}$ is symmetric and if we consider a symmetric configuration in coordinate space, i.e. the three particles are located at the vertices of an equilateral triangle, then the function $\phi^{\beta}_{[i]}$ is symmetric for exchange of particles and, therefore, the $\ell_1 = \ell_2 = 0$ component of the wave function must vanish for this specific configuration. Therefore, we expect this channel to be suppressed. Similarly, for $t_\beta = 1/2$ and $j^\pi = \frac{3}{2}^+$, the $\ell_1 = \ell_2 = 0$ component comes with a $s = 3/2$ symmetric function. Therefore, this component must vanish for equilateral-triangle configuration and this channel is

also expected to be suppressed. This is similar to the arguments presented in the paper based on the Pauli exclusion rule considering three particles in the same location. Therefore, we are eventually left with a single dominant channel at short distances corresponding to $t_\beta = 1/2$, $j_\beta = \frac{1}{2}$, $\pi_\beta = +$ (and $m_\beta = \pm 1/2$ and $t_{z,\beta} = \pm 1/2$)

## II. PROPERTIES OF THE THREE-BODY NUCLEAR CONTACTS

### A. Non-averaged contacts

Considering the asymptotic three-nucleon factorization, and in order to ensure that the many-body wave function $\Psi$ has a total angular momentum $J$ and projection $M$, the $B_{ijl}^{\beta}$ functions are given by

$$B_{ijl}^{\beta}\left(\boldsymbol{R}_{ijl}, \{\boldsymbol{r}_k\}_{k\neq i,j,l}\right) = \sum_{J_{A-3},M_{A-3}} \langle j_\beta m_\beta J_{A-3} M_{A-3} | JM\rangle B_{ijl}^{\{\pi_\beta, j_\beta, t_\beta, t_{z,\beta}\} J_{A-3}, M_{A-3}}\left(\boldsymbol{R}_{ijl}, \{\boldsymbol{r}_k\}_{k\neq i,j,l}\right) , \tag{4}$$

where $J_{A-3}$ and $M_{A-3}$ are the angular momentum quantum numbers with respect to the sum $\boldsymbol{J}_{A-3} + \boldsymbol{L}_{3,CM}$ of the intrinsic angular momentum of the residual $(A-3)$ particles $\boldsymbol{J}_{A-3}$, and the orbital angular momentum $\boldsymbol{L}_{3,CM}$ corresponding to $\boldsymbol{R}_{ijl}$. $B_{ijl}^{\{\pi_\beta, j_\beta, t_\beta, t_{z,\beta}\} J_{A-3}, M_{A-3}}$ is a set of functions with angular momentum quantum numbers $J_{A-3}$ and $M_{A-3}$, which depends also on the numbers $\pi_\beta, j_\beta, t_\beta, t_{z,\beta}$. $\langle j_\beta m_\beta J_{A-3} M_{A-3} | JM\rangle$ are the Clebsch-Gordan coefficients. The sum over $M_{A-3}$ in Eq. (4) together with the sum over $m_\beta$ that is included in the sum over $\beta$ in the asymptotic factorization guarantee that $\Psi$ has well-defined $J$ and $M$ quantum numbers.

Based on this expression for $B_{ijl}^{\beta}$ we can see directly that $C_3^{\beta\gamma}(JM) = 0$ if $m_\beta \neq m_\gamma$ due to the orthogonality of $B_{ijl}^{\{\pi_\beta, j_\beta, t_\beta, t_{z,\beta}\} J_{A-3}, M_{A-3}}$ in $M_{A-3}$. We can similarly conclude that $C_3^{\beta\gamma}(JM) = 0$ if $t_{z,\beta} \neq t_{z,\gamma}$ assuming $\Psi$ has good isospin quantum numbers. If $\Psi$ is an eigenstate of the Hamiltonian, it has well-defined parity and, therefore, the parity of $\varphi_{ijl}^{\beta}$ dictates the parity of $B_{ijl}^{\beta}$. In this case we also get that $C_3^{\beta\gamma}(JM) = 0$ if $\pi_\beta \neq \pi_\gamma$. For $J = 0$ nuclei, $J_{A-3}$ must be equal to $j_\beta$ and therefore $C_3^{\beta\gamma}(00) = 0$ if $j_\beta \neq j_\gamma$ due to the orthogonality of $B_{ijl}^{\{\pi_\beta, j_\beta, t_\beta, t_{z,\beta}\} J_{A-3}, M_{A-3}}$ in $J_{A-3}$. Similarly, for $T = 0$ nuclei, $C_3^{\beta\gamma}(JM) = 0$ if $t_\beta \neq t_\gamma$.

Finally, we claimed in the paper that the sum over $m_\beta$ of the diagonal contacts $\sum_{m_\beta} C_3^{\beta\beta}(JM)$ is independent of M. We provide a short proof here. Using Eq. (4) and the definition of the contacts we obtain

$$\sum_{m_\beta} C_3^{\beta\beta}(JM) = \binom{A}{3} \sum_{m_\beta} \sum_{J_{A-3},M_{A-3}} |\langle j_\beta m_\beta J_{A-3} M_{A-3} | JM\rangle|^2 \langle B_{ijl}^{\{\pi_\beta, j_\beta, t_\beta, t_{z,\beta}\} J_{A-3}, M_{A-3}} | B_{ijl}^{\{\pi_\beta, j_\beta, t_\beta, t_{z,\beta}\} J_{A-3}, M_{A-3}}\rangle. \tag{5}$$

We used here the orthogonality of $B_{ijl}^{\{\pi_\beta, j_\beta, t_\beta, t_{z,\beta}\} J_{A-3}, M_{A-3}}$ in $J_{A-3}$ and $M_{A-3}$. Based on the Wigner Eckart theorem, the last matrix element above does not depend on $M_{A-3}$. Thus,

$$\sum_{m_\beta} C_3^{\beta\beta}(JM) = \binom{A}{3} \sum_{J_{A-3}} \langle B_{ijl}^{\{\pi_\beta, j_\beta, t_\beta, t_{z,\beta}\} J_{A-3}} || B_{ijl}^{\{\pi_\beta, j_\beta, t_\beta, t_{z,\beta}\} J_{A-3}}\rangle \sum_{m_\beta} \sum_{M_{A-3}} |\langle j_\beta m_\beta J_{A-3} M_{A-3} | JM\rangle|^2. \tag{6}$$

The double sum of the Clebsch-Gordan coefficients is equal to one, due to their orthogonality properties, and we get here an $M$-independent quantity.

### B. $M$-averaged contacts

We prove in this section the orthogonality of the M-averaged contacts in $j$, and also that these averaged contacts are independent of $m$. Using Eq. (4) and the definition of the averaged contacts we obtain

$$C_3^{\beta\gamma} = \binom{A}{3} \frac{1}{2J+1} \sum_{J_{A-3}} \langle B_{ijl}^{\{\pi_\beta, j_\beta, t_\beta, t_{z,\beta}\} J_{A-3}} || B_{ijl}^{\{\pi_\gamma, j_\gamma, t_\gamma, t_{z,\gamma}\} J_{A-3}}\rangle \sum_{M} \sum_{M_{A-3}} \langle j_\beta m_\beta J_{A-3} M_{A-3} | JM\rangle^* \langle j_\gamma m_\gamma J_{A-3} M_{A-3} | JM\rangle. \tag{7}$$

As in the derivation above, we used here the orthogonality of $B_{ijl}^{\{\pi_\beta, j_\beta, t_\beta, t_{z,\beta}\} J_{A-3}, M_{A-3}}$ in $J_{A-3}$ and $M_{A-3}$, and the independence of the matrix element $\langle B_{ijl}^{\{\pi_\beta, j_\beta, t_\beta, t_{z,\beta}\} J_{A-3}, M_{A-3}} | B_{ijl}^{\{\pi_\gamma, j_\gamma, t_\gamma, t_{z,\gamma}\} J_{A-3}, M_{A-3}}\rangle$ of $M_{A-3}$ and $M$. Using now

the Clebsch-Gordan identity

$$\langle j_1 m_1 j_2 m_2 | j_3 m_3 \rangle = (-1)^{j_2+m_2} \left( \frac{2j_3+1}{2j_1+1} \right)^{1/2} \langle j_2 - m_2 j_3 m_3 | j_1 m_1 \rangle \tag{8}$$

for the two Clebsch-Gordan coefficients we get

$$C_3^{\beta\gamma} = \binom{A}{3} \frac{1}{2J+1} \left( \frac{2J+1}{2j_\beta+1} \right)^{1/2} \left( \frac{2J+1}{2j_\gamma+1} \right)^{1/2} \sum_{J_{A-3}} \langle B_{ijl}^{\{\pi_\beta, j_\beta, t_\beta, t_{z,\beta}\} J_{A-3}} || B_{ijl}^{\{\pi_\gamma, j_\gamma, t_\gamma, t_{z,\gamma}\} J_{A-3}} \rangle$$
$$\times \sum_M \sum_{M_{A-3}} (-1)^{2(J_{A-3}+M_{A-3})} \langle j_\beta m_\beta | J_{A-3} - M_{A-3} JM \rangle \langle J_{A-3} - M_{A-3} JM | j_\gamma m_\gamma \rangle. \tag{9}$$

$J_{A-3}+M_{A-3}$ is an integer so $(-1)^{2(J_{A-3}+M_{A-3})} = 1$, and this allows us to use the orthogonality of the Clebsch-Gordan coefficients and get

$$C_3^{\beta\gamma} = \delta_{j_\beta j_\gamma} \delta_{m_\beta m_\gamma} \binom{A}{3} \frac{1}{2j_\beta+1} \sum_{J_{A-3}} \langle B_{ijl}^{\{\pi_\beta, j_\beta, t_\beta, t_{z,\beta}\} J_{A-3}} || B_{ijl}^{\{\pi_\gamma, j_\gamma, t_\gamma, t_{z,\gamma}\} J_{A-3}} \rangle. \tag{10}$$

We can clearly see that indeed the averaged contacts are diagonal in $j$ and $m$, and also are independent of $m$.
